# Supplementary material for: RAG-Star: Enhancing Deliberative Reasoning with Retrieval Augmented Verification and Refinement
Source: arXiv:2412.12881 source file (2024-12-17)
Supplement: Supplementary file 1 [file sec-appendix.tex]

\clearpage
\appendix
\label{appendix}

\section{Experiment Setup}
\label{sec:app-experiment}
\subsection{Datasets}

\subsection{Evaluation Protocol} 

\subsection{Baselines for Comparison}

\subsection{Implementation Details}

\section{Summary of Toolbox}
\label{sec:app-tool}
